# Supplementary material for: Shape-Graph Matching Network (SGM-net): Registration for Statistical Shape Analysis
Source: arXiv:2308.06869 source file (2023-08-14)

**Ours**

**FGM**

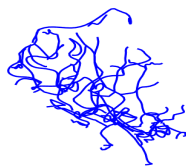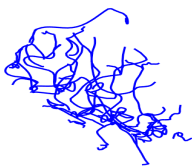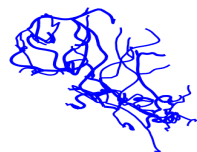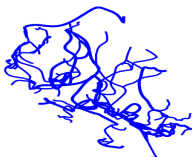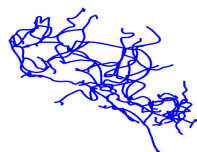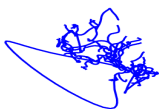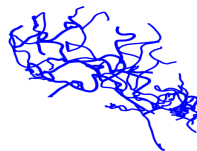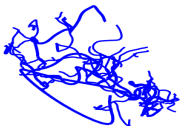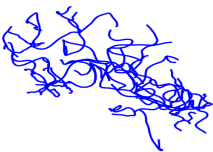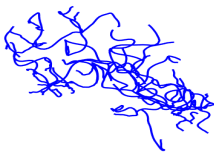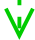

Supplement: Supplementary file 1 [file geo_ban.pdf]
